# Supplementary material for: TLIO: Tight Learned Inertial Odometry
Source: arXiv:2007.01867 source file (2020-07-10)
Supplement: Supplementary file 1 [file appendix.tex]

\subsection{State Propagation}

The state propagation Eq.~\ref{eq:kf-prop} is the following:
\begin{align*}
&\tilde{s}_{k+1} = A_k^s \tilde{s}_k + B_k^s n_{IMU} + C_k^s \eta \\
&\tilde{s}_{k+1} = \begin{bmatrix}
\errr_{k+1}\\ \errv_{k+1}\\ \errp_{k+1}\\ \errb_{g(k+1)}\\ \errb_{a(k+1)}
\end{bmatrix} =
\begin{bmatrix}
\Ib & \zerob & \zerob & -\hat{R}_{k+1}J_r((\omega_k-\hat{b}_{gk})\Delta t)\Delta t & \zerob\\
-\floor{\hat{R}_k(a_k-\hat{b}_{ak})}_{\times} \Delta t & \Ib & \zerob & \zerob & -\hat{R}_k \Delta t\\
-\frac{1}{2}\floor{\hat{R}_k(a_k-\hat{b}_{ak})}_{\times} \Delta t^2 & \Ib\Delta t & \Ib & \zerob & -\frac{1}{2}\hat{R}_k \Delta t^2\\
\zerob & \zerob & \zerob & \Ib & \zerob\\
\zerob & \zerob & \zerob & \zerob & \Ib
\end{bmatrix} \begin{bmatrix}
\errr_k\\ \errv_k\\ \errp_k\\ \errb_{gk}\\ \errb_{ak}
\end{bmatrix}\\
&+ \begin{bmatrix}
\hat{R}_{k+1}J_r((\omega_k - \hat{b}_{gk})\Delta t)\Delta t & \zerob\\
\zerob & \hat{R}_k \Delta t\\
\zerob & \frac{1}{2}\hat{R}_k\Delta t^2\\
\zerob & \zerob\\
\zerob & \zerob
\end{bmatrix} \begin{bmatrix}
n_{\omega k}\\ n_{ak}
\end{bmatrix} + \begin{bmatrix}
\zerob & \zerob\\
\zerob & \zerob\\
\zerob & \zerob\\
\Ib & \zerob\\
\zerob & \Ib
\end{bmatrix} \begin{bmatrix}
\eta_{gdk}\\ \eta_{adk}
\end{bmatrix}
\end{align*}
$J_r$ is the right Jacobian of $SO(3)$.

\subsection{Measurement Update}

The proof of $H_{\errr_i}$ in Eq.~\ref{eq:kf-meas} is as follows:

\begin{proof}
According to chain rule,
\begin{equation}
H_{\errr_i} = \frac{\partial h(X)}{\partial \theta_i} = \frac{\partial h(X)}{\partial \theta_{iz}} \cdot \frac{\partial \theta_{iz}}{\partial r} \cdot \frac{\partial r}{\partial \theta_i} \label{eq:app-chain}
\end{equation}
where $\theta_{iz}$ is the vector form of $\sof(3)$ of the rotation matrix $R_{iz}$, defined as $\text{Log}(R_{iz})$, and $\theta_i = \text{Log}(R_i)$. $r$ is defined as $(\alpha, \beta, \gamma)^T$ where $\alpha$, $\beta$ and $\gamma$ corresponds to yaw, pitch and roll angles of the $R_i$ respectively:
\begin{align*}
R_i(\alpha,\beta,\gamma) &= R_{\alpha \ibb} R_{\beta \jbb} R_{\gamma \kbb} = \begin{bmatrix}
\cos{\alpha} & -\sin{\alpha} & 0\\
\sin{\alpha} & \cos{\alpha} & 0\\
0 & 0 & 1
\end{bmatrix} \begin{bmatrix}
\cos{\beta} & 0 & \sin{\beta} \\
0 & 1 & 0\\
-\sin{\beta} & 0 & \cos{\beta}
\end{bmatrix} \begin{bmatrix}
1 & 0 & 0 \\
0 & \cos{\gamma} & -\sin{\gamma}\\
0 & \sin{\gamma} & \cos{\gamma}
\end{bmatrix},\\
&\text{where } \ibb=(0,0,1)^T \text{, }\jbb =(0,1,0)^T \text{, }\kbb =(1,0,0)^T
\text{, and } R_{\alpha \ibb} = R_{iz}
\end{align*}

According to \cite{trawny2005jacobian}, we have
\begin{align*}
H = \frac{\partial \theta_i}{\partial r} = \begin{bmatrix}
\ibb & R_{\alpha \ibb} \jbb & R_{\alpha \ibb} R_{\beta \jbb} \kbb
\end{bmatrix} = \begin{bmatrix}
0 & -\sin{\alpha} & \cos{\alpha}\sin{\beta} \\
0 & \cos{\alpha} & \sin{\alpha}\cos{\beta} \\
1 & 0 & -\sin{\beta}
\end{bmatrix}
\end{align*}
and we have $det(H) = -\cos{\beta}$. Singularity occurs when $\beta = \pm \frac{\pi}{2}$ and is known as gimbal lock.

From the inverse function theorem, when $det(H) \neq 0$, we have 
\begin{align*}
\frac{\partial r}{\partial \theta_i} = H^{-1} = \begin{bmatrix}
\cos{\alpha}\tan{\beta} & \sin{\alpha}\tan{\beta} & 1\\
-\sin{\alpha} & \cos{\alpha} & 0\\
\cos{\alpha}\sec{\beta} & \sec{\beta}\sin{\alpha} & 0
\end{bmatrix}
\end{align*}
where $H^{-1}$ has a closed form solution. This is the last term of the chain rule in Eq.~\ref{eq:app-chain}.

The second term can be easily obtained as $\theta_{iz} = \text{Log}(R_iz) = (0,0,\alpha)^T$:
\begin{align*}
\frac{\partial \theta_{iz}}{\partial r} = \begin{bmatrix}
0 & 0 & 0\\
0 & 0 & 0\\
1 & 0 & 0
\end{bmatrix}
\end{align*}

To obtain the first term we use the same technique for calculating the state propagation matrix, where we expand $h(X)$ by $\errr{iz}$:
\begin{align*}
\delta h(X) &= (e^{\errr{iz}} R_{iz})^T (p_j - p_i)\\
&=R_{iz}^T e^{-\errr_{iz}} (p_j - p_i)\\
&=R_{iz}^T (\Ib - \floor{\errr_{iz}}_{\times}) (p_j - p_i)\\
&=R_{iz}^T (p_j - p_i) - R_{iz}^T \floor{\errr_{iz}}_{\times}  (p_j - p_i) \\
&=R_{iz}^T (p_j - p_i) - R_{iz}^T \floor{(p_j - p_i)}_{\times} \errr_{iz}
\end{align*}
So we have
\begin{align*}
\frac{\partial h(X)}{\partial \theta_{iz}} = - R_{iz}^T \floor{(p_j - p_i)}_{\times} 
\end{align*}

Therefore,
\begin{align*}
H_{\errr_i} &= \frac{\partial h(X)}{\partial \theta_i} =\frac{\partial h(X)}{\partial \theta_{iz}} \cdot \frac{\partial \theta_{iz}}{\partial r} \cdot \frac{\partial r}{\partial \theta_i} \\
&= \hat{R}_{iz}^T \floor{\hat{p}_j-\hat{p}_i}_{\times} \begin{bmatrix}
0 & 0 & 0\\
0 & 0 & 0\\
1 & 0 & 0
\end{bmatrix} \begin{bmatrix}
\cos{\alpha}\tan{\beta} & \sin{\alpha}\tan{\beta} & 1\\
-\sin{\alpha} & \cos{\alpha} & 0\\
\cos{\alpha}\sec{\beta} & \sec{\beta}\sin{\alpha} & 0
\end{bmatrix}\\
&=\hat{R}_{iz}^T \floor{\hat{p}_j-\hat{p}_i}_{\times}
\begin{bmatrix}
0 & 0 & 0\\
0 & 0 & 0\\
\cos{\alpha}\tan{\beta} & \sin{\alpha}\tan{\beta} & 1
\end{bmatrix}
\end{align*}

\end{proof}
